# Supplementary material for: RoboCrowd: Scaling Robot Data Collection through Crowdsourcing
Source: arXiv:2411.01915 source file (2025-05-21)

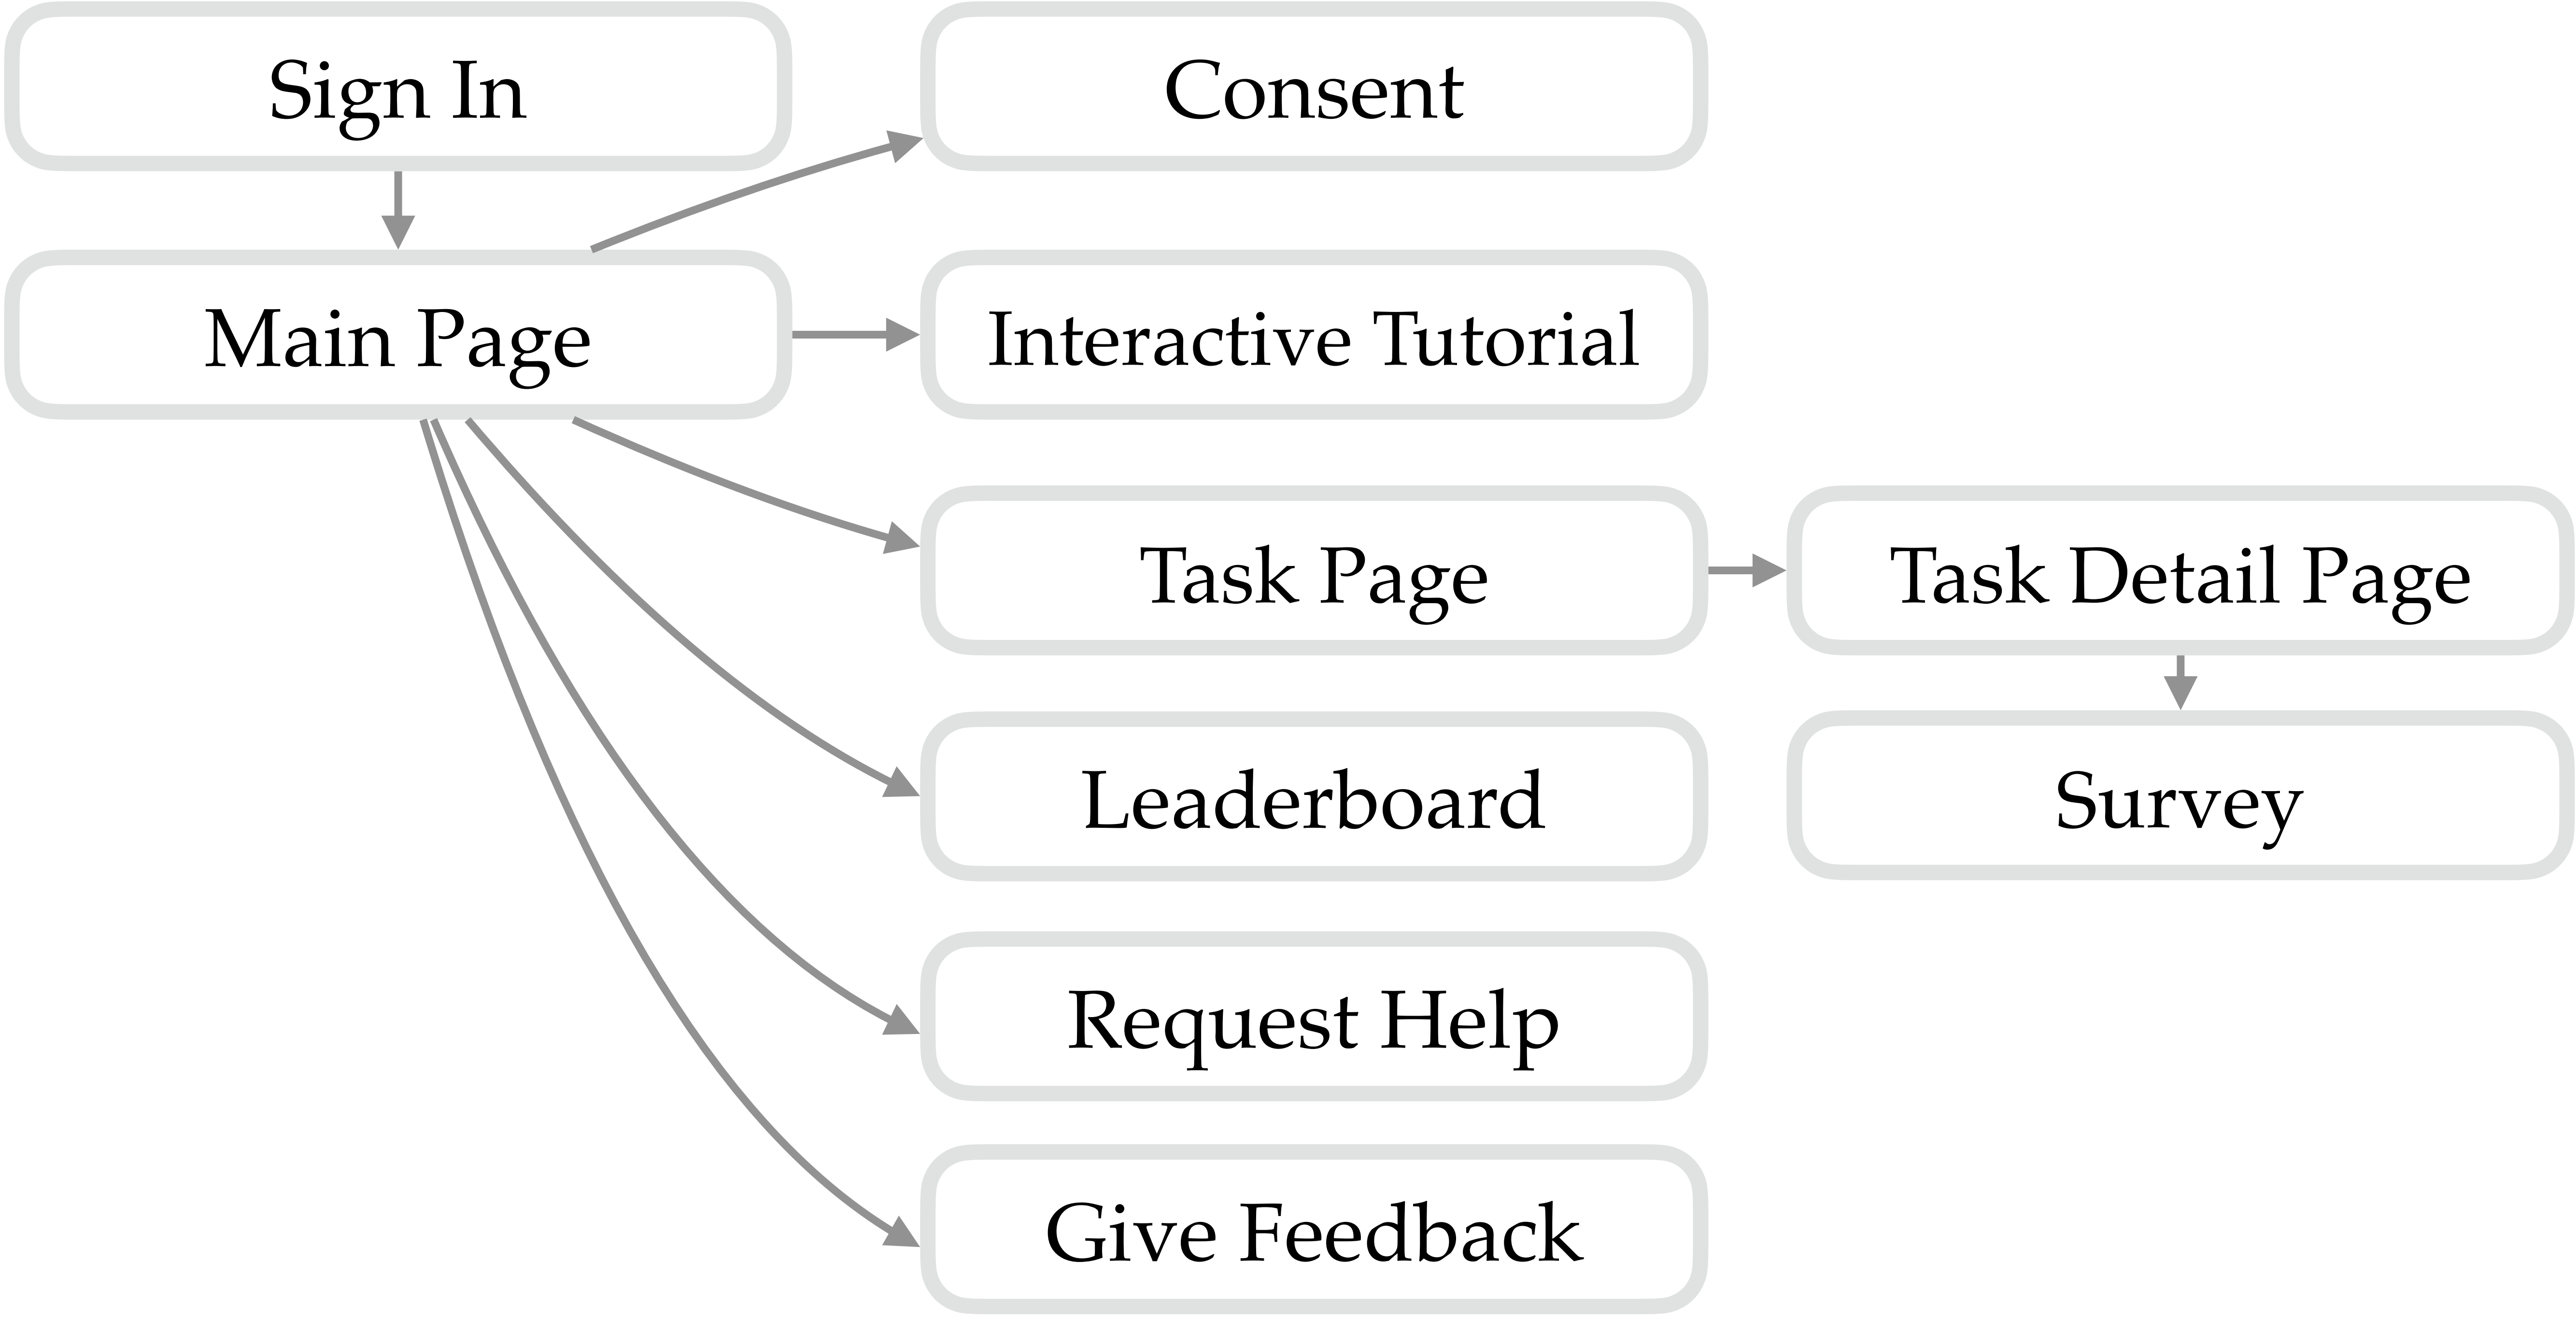
Sign In
Consent
Main Page
Interactive Tutorial
Task Page
Task Detail Page
Leaderboard
Survey
Request Help
Give Feedback

Tap your [illegible] ID on the card reader to begin

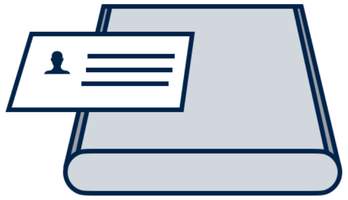

REQUEST HELP

# Play With ALOHA

Welcome! Type a nickname below to get started.

May be displayed on leaderboard

Your nickname

GET STARTED

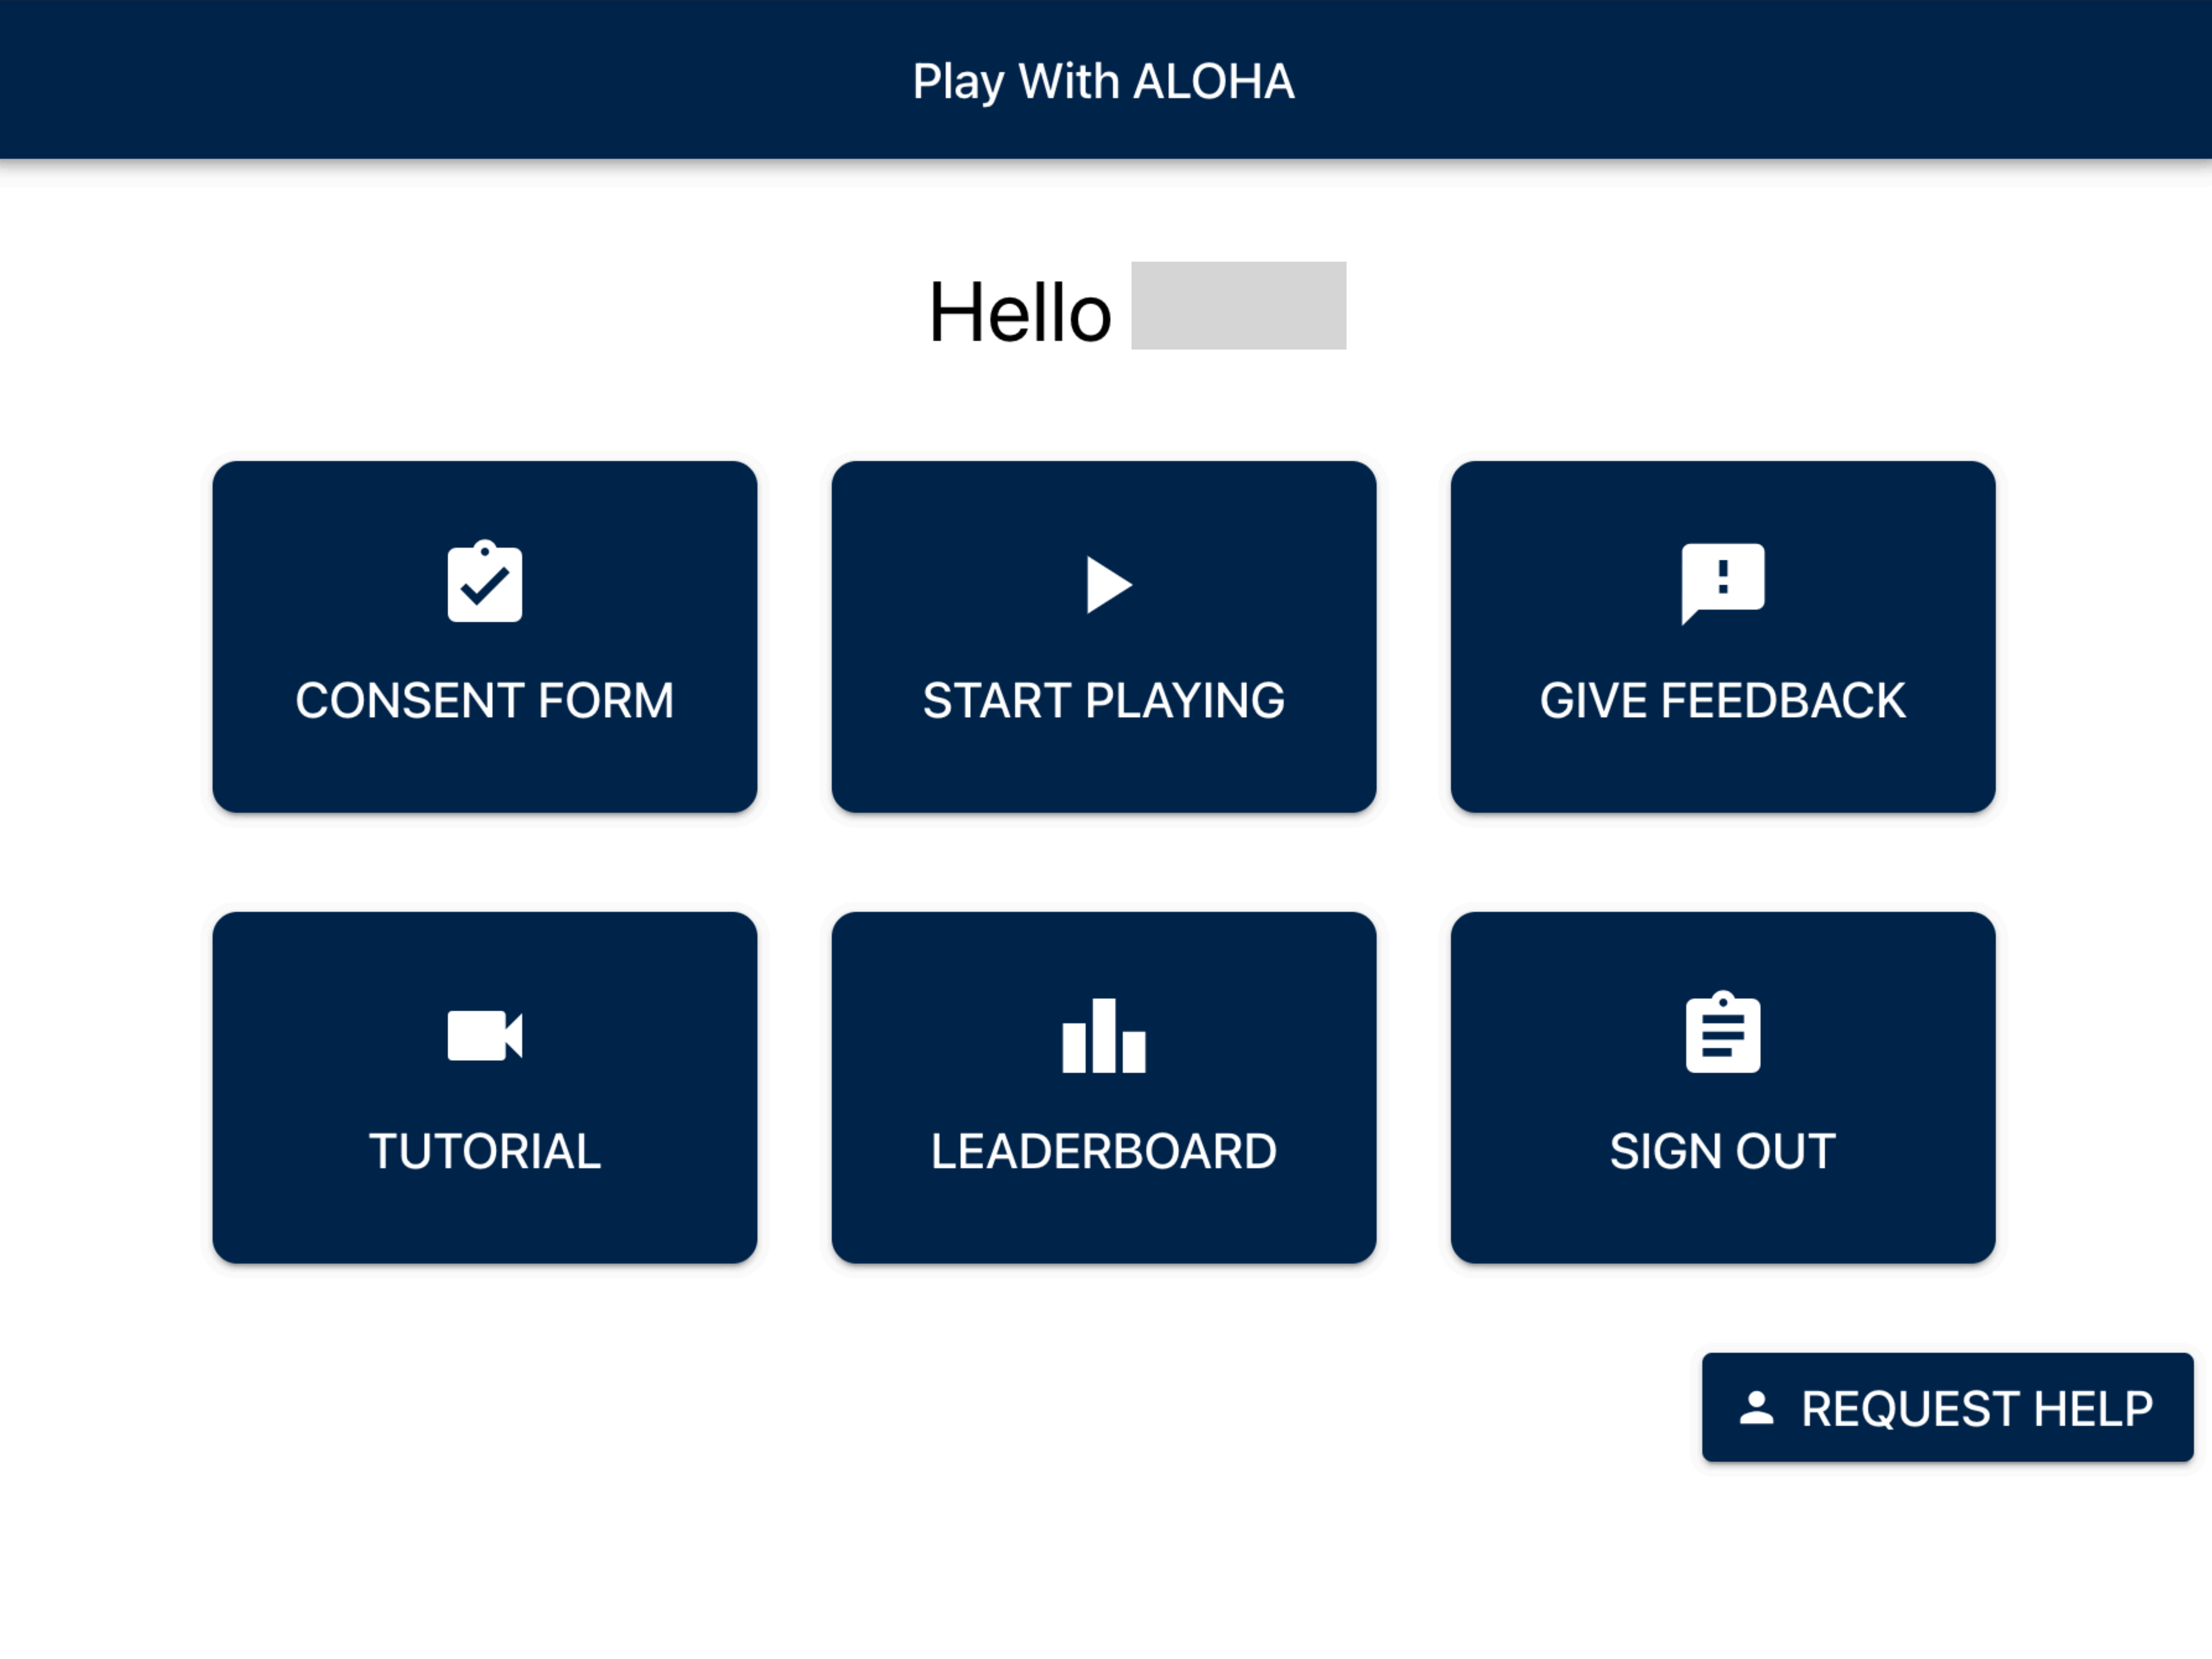
Play With ALOHA
Hello
CONSENT FORM
START PLAYING
GIVE FEEDBACK
TUTORIAL
LEADERBOARD
SIGN OUT
REQUEST HELP

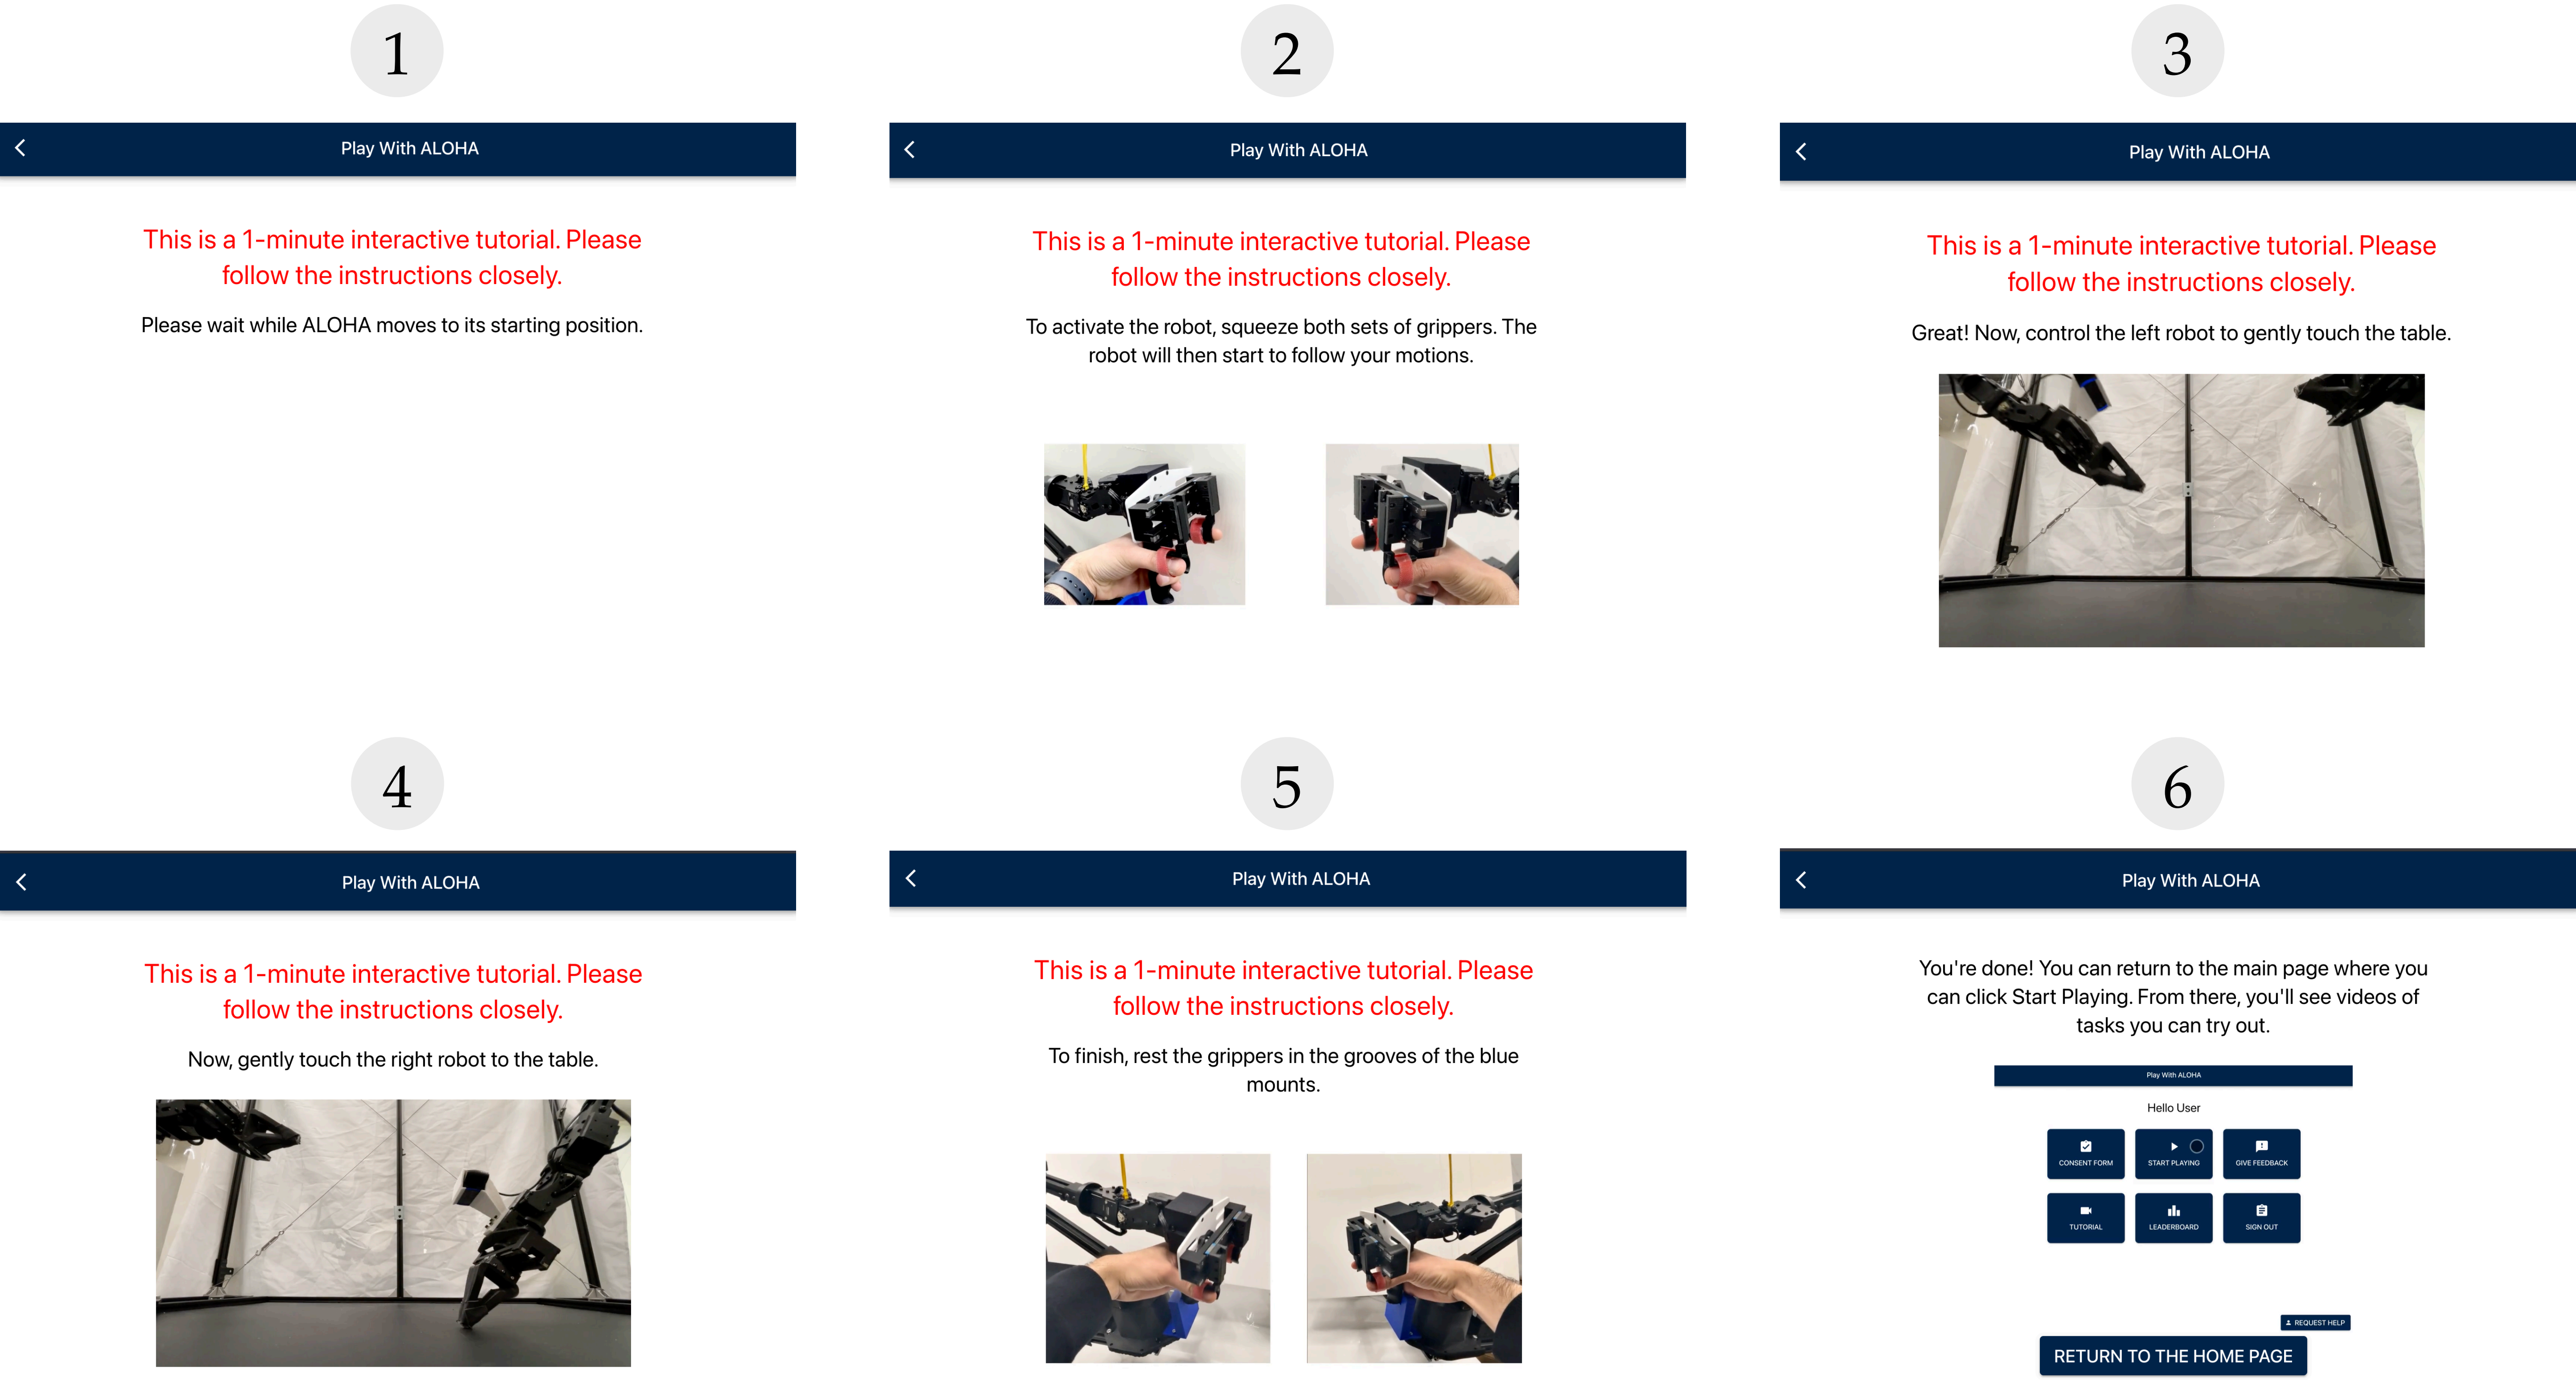
1
Play With ALOHA
This is a 1-minute interactive tutorial. Please follow the instructions closely.
Please wait while ALOHA moves to its starting position.
2
Play With ALOHA
This is a 1-minute interactive tutorial. Please follow the instructions closely.
To activate the robot, squeeze both sets of grippers. The robot will then start to follow your motions.
3
Play With ALOHA
This is a 1-minute interactive tutorial. Please follow the instructions closely.
Great! Now, control the left robot to gently touch the table.
4
Play With ALOHA
This is a 1-minute interactive tutorial. Please follow the instructions closely.
Now, gently touch the right robot to the table.
5
Play With ALOHA
This is a 1-minute interactive tutorial. Please follow the instructions closely.
To finish, rest the grippers in the grooves of the blue mounts.
6
Play With ALOHA
You're done! You can return to the main page where you can click Start Playing. From there, you'll see videos of tasks you can try out.
Play With ALOHA
Hello User
CONSENT FORM
START PLAYING
GIVE FEEDBACK
TUTORIAL
LEADERBOARD
SIGN OUT
REQUEST HELP
RETURN TO THE HOME PAGE

Play With ALOHA

# Choose a Task

## (Easy) Pick up a Hi-Chew from a bin

Pick up a Hi-Chew from a bin, and bring it to the End Zone

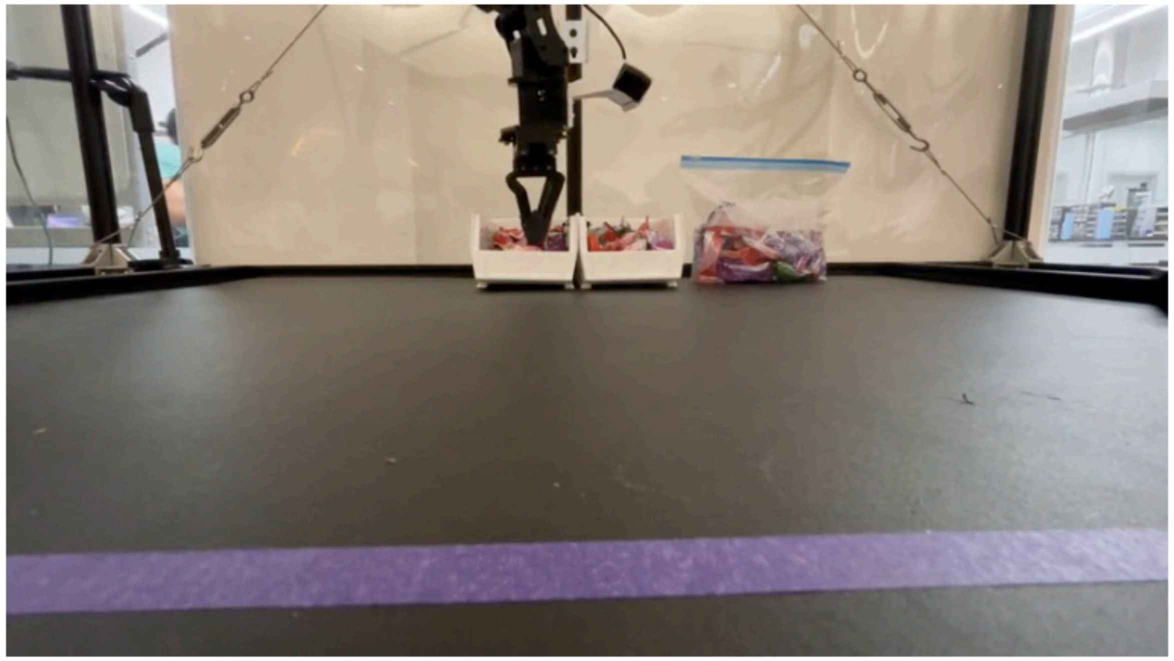

PLAY

## (Hard) Open Ziploc, then grab a Hi-Chew, then close Ziploc

Unzip the Ziploc bag, then grab a Hi-Chew and bring it to the End Zone. Then, re-zip the Ziploc.

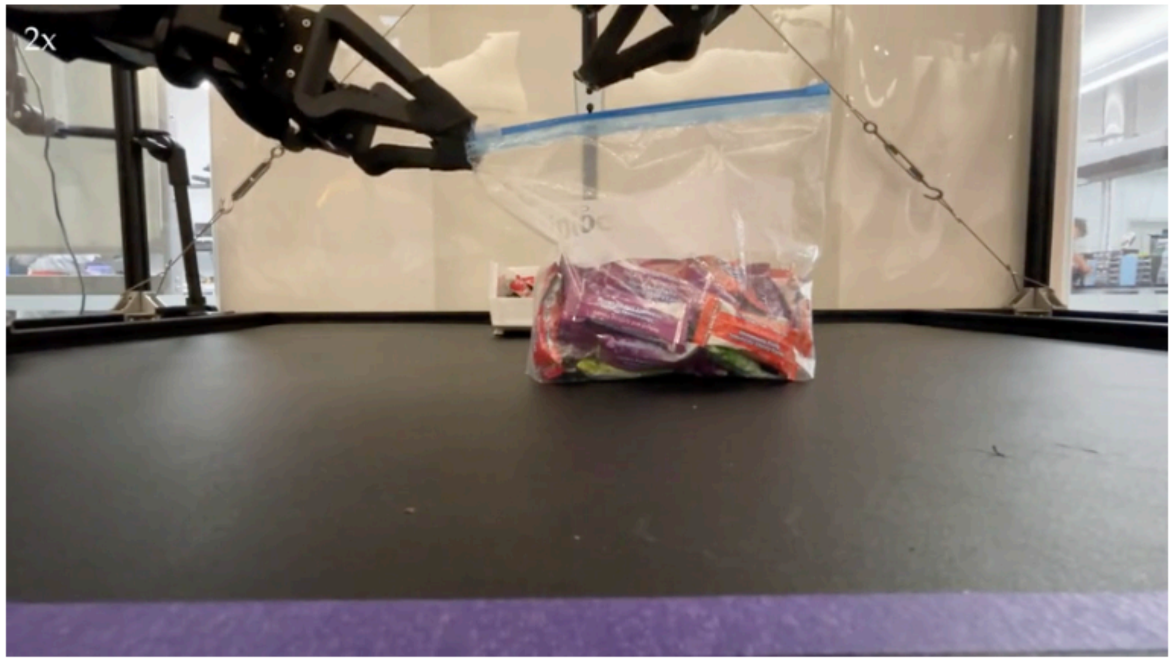


PLAY

# (Hard) Open Ziploc, then grab a Hi-Chew, then close Ziploc

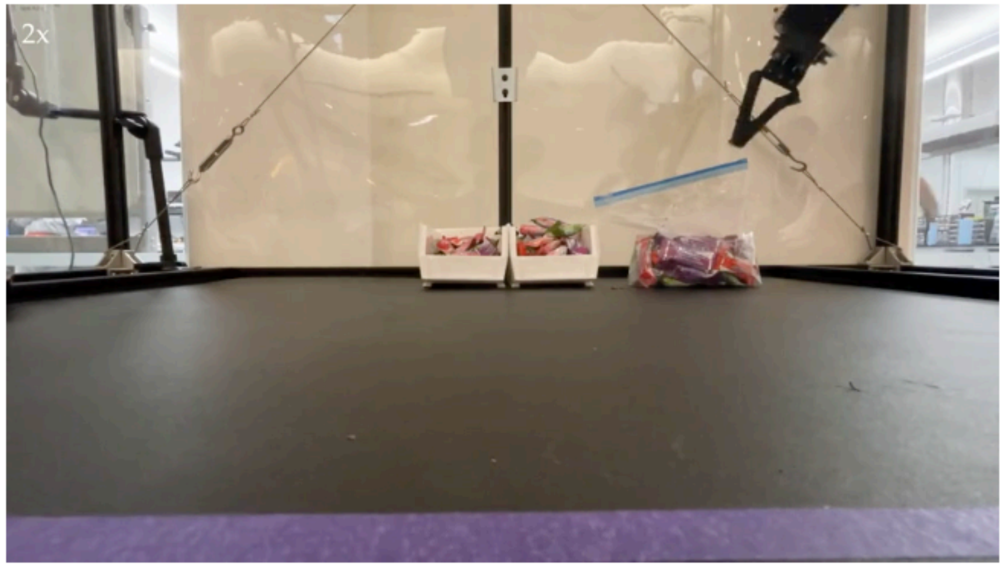


### Description:

Unzip the Ziploc bag, then grab a Hi-Chew and bring it to the End Zone. Then, re-zip the Ziploc.

### Instructions:

To start your demonstration, click the Start button and then squeeze ALOHA's grippers until they are closed.

To stop the demonstration, rest ALOHA's grippers down and click the Stop button.

START

STOP

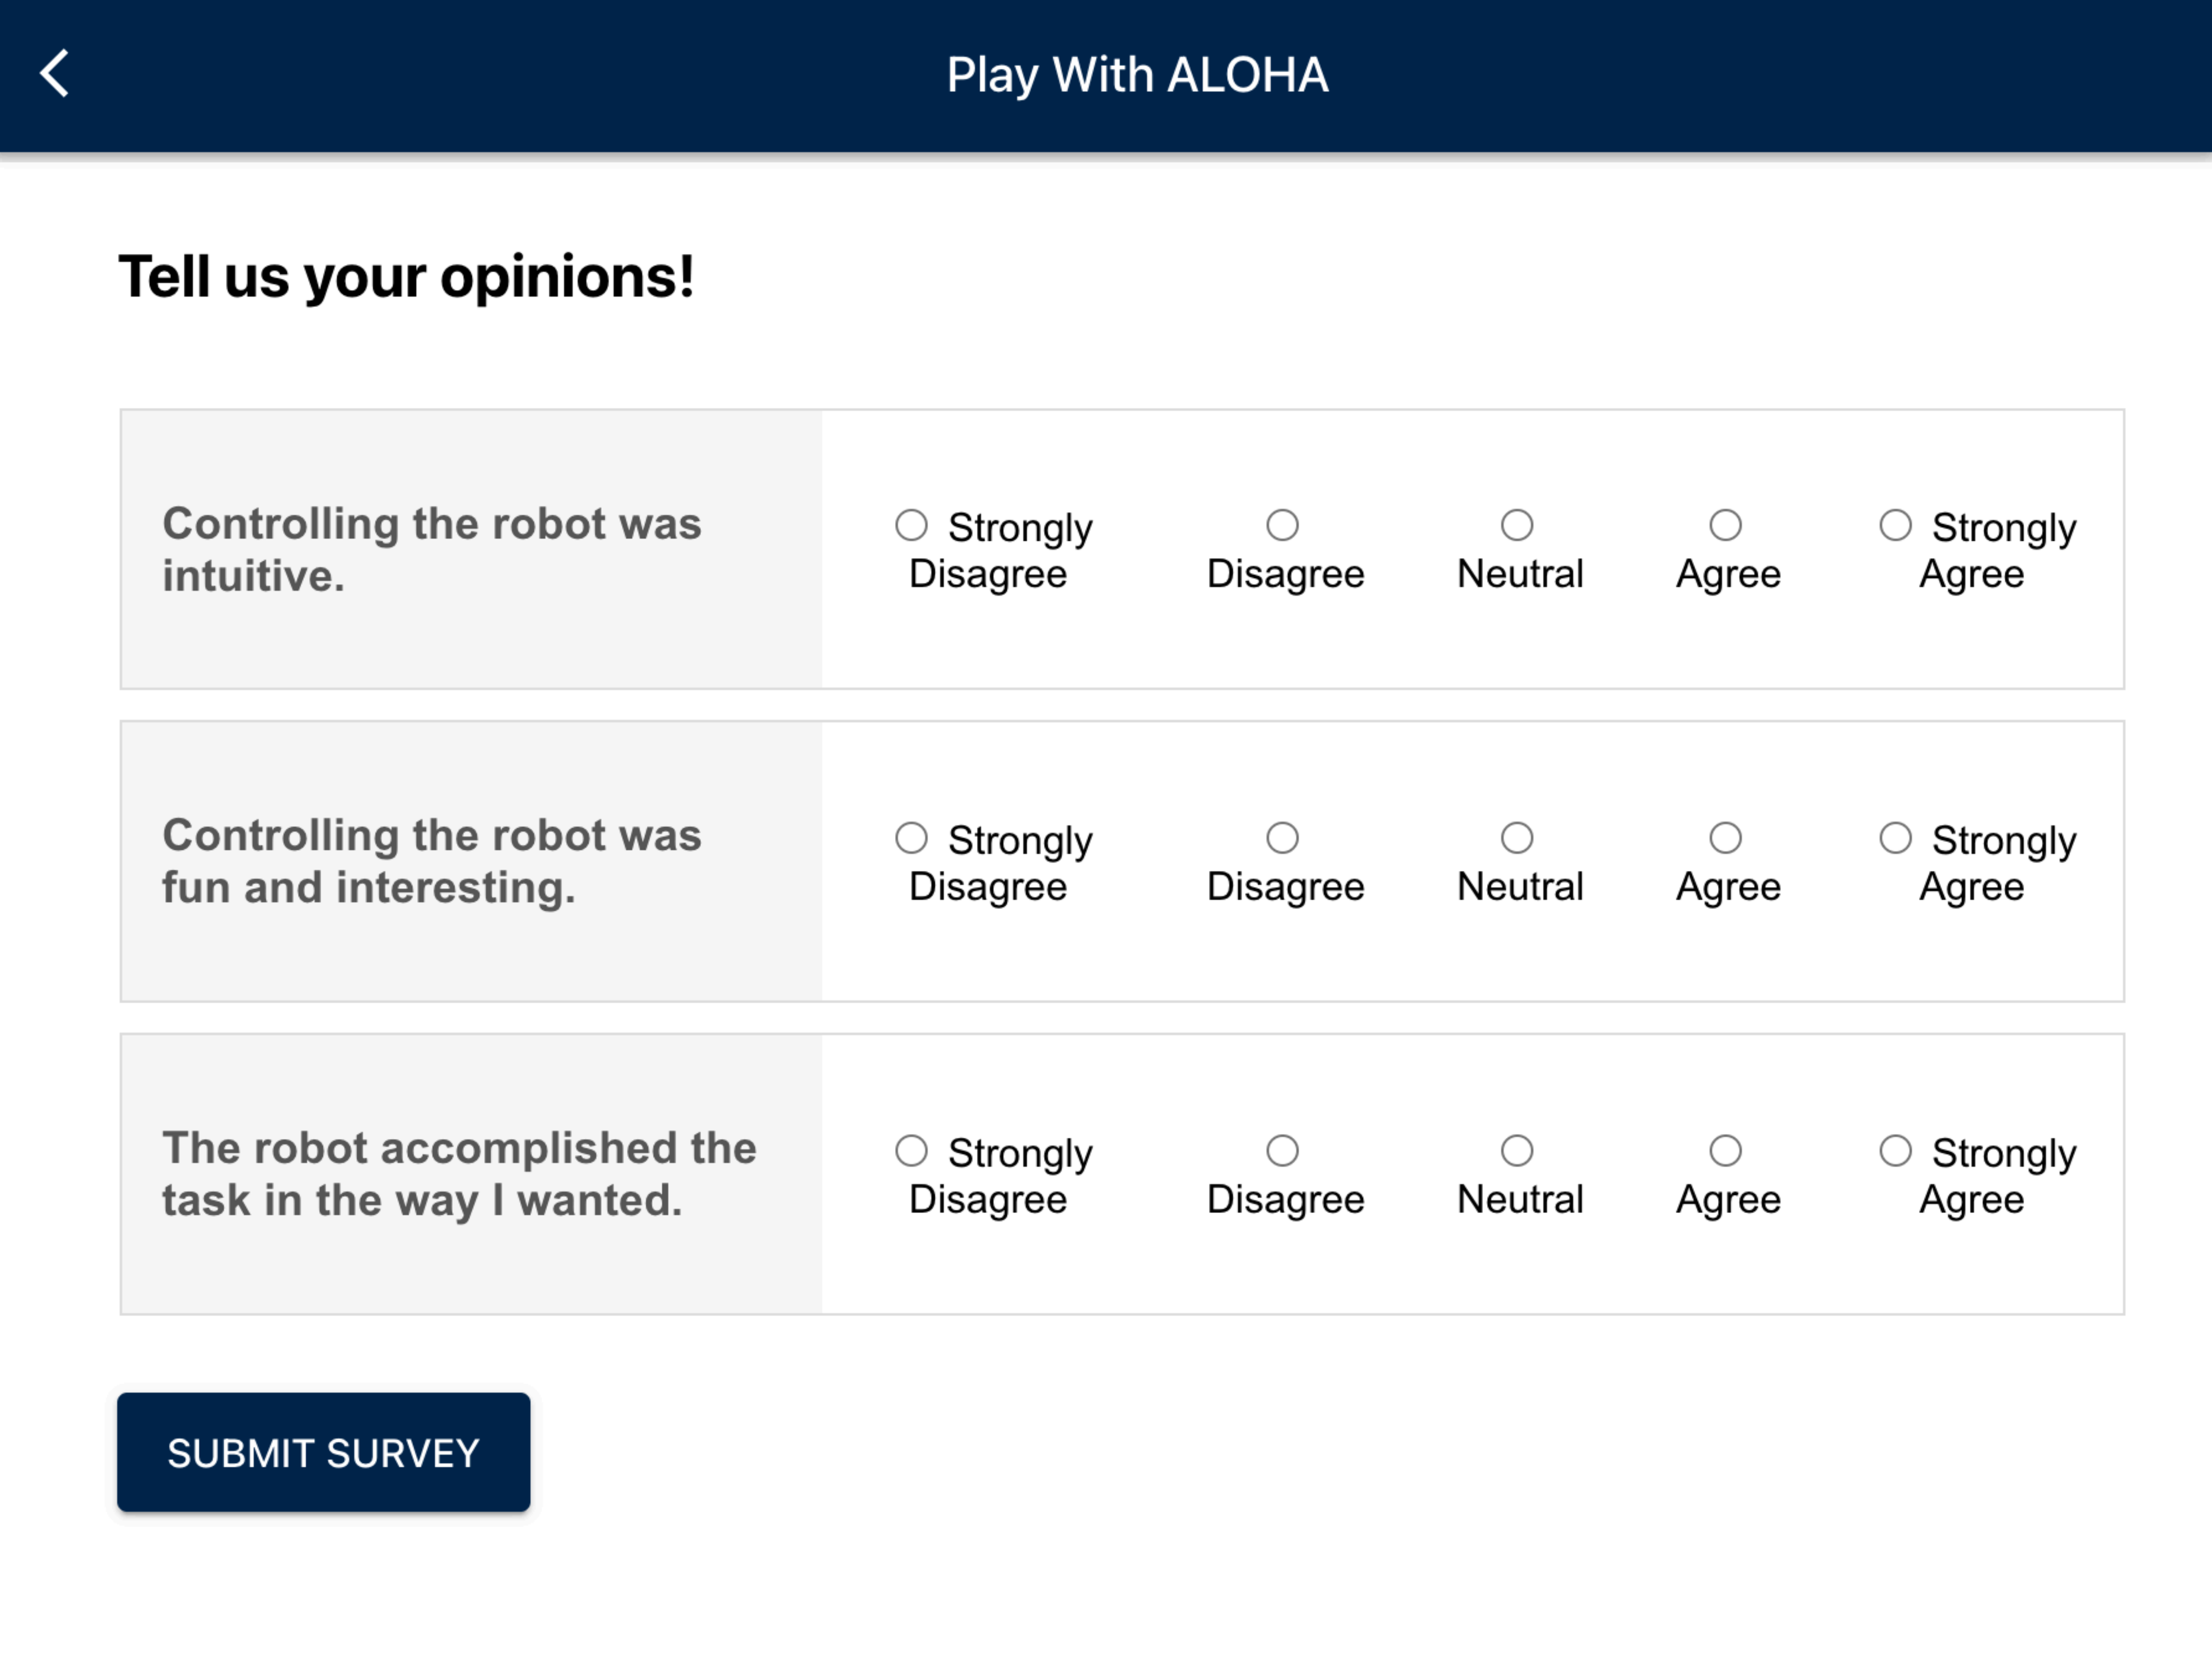
Play With ALOHA
Tell us your opinions!
Controlling the robot was intuitive.
Strongly Disagree
Disagree
Neutral
Agree
Strongly Agree
Controlling the robot was fun and interesting.
Strongly Disagree
Disagree
Neutral
Agree
Strongly Agree
The robot accomplished the task in the way I wanted.
Strongly Disagree
Disagree
Neutral
Agree
Strongly Agree
SUBMIT SURVEY

Play With ALOHA

# Leaderboard

| Rank | Name | Score |
|---|---|---|
| 1 | | 640 |
| 2 | | 390 |
| 3 | | 260 |
| 4 | | 170 |
| 5 | | 130 |
| 6 | | 130 |
| 7 | | 120 |
| 8 | | 120 |

Optionally, describe the issue here.

REQUEST HELP

Play With ALOHA

Feedback

SUBMIT FEEDBACK

Careful! ALOHA's arms are near collision

# (Hard) Open Ziploc, then grab a Hi-Chew, then close Ziploc

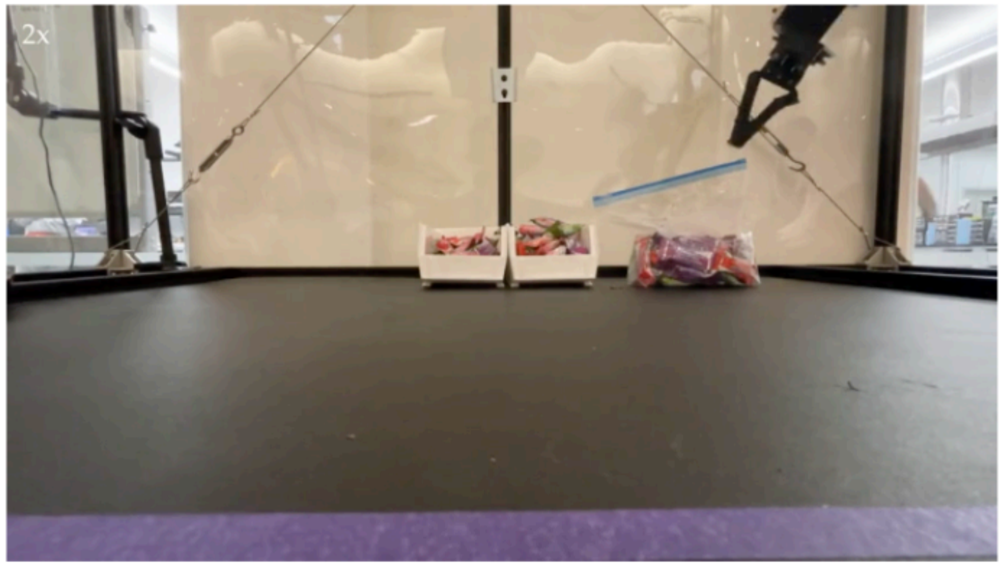

## Description:

Unzip the Ziploc bag, then grab a Hi-Chew and bring it to the End Zone. Then, re-zip the Ziploc.

## Instructions:

To start your demonstration, click the Start button and then squeeze ALOHA's grippers until they are closed.

To stop the demonstration, rest ALOHA's grippers down and click the Stop button.

START

STOP

< | > | Flag | Change | play - 1 | Reset | Commit | Prev Episode | Next Episode

Image Index 24

**Episode Index:**5

**Image Index:** 24

**Current Label:** play - 1

**Flags:** [8, 8, 8, 8, 8, 8, 8, 8, 8, 8, 8, 0, 0, 0, 0, 0, 0, 0, 0, 0, 0, 0, 0, 0, 0, 0, 0, 0, 0, 0, 0, 0, 0, 0, 0, 0, 0]

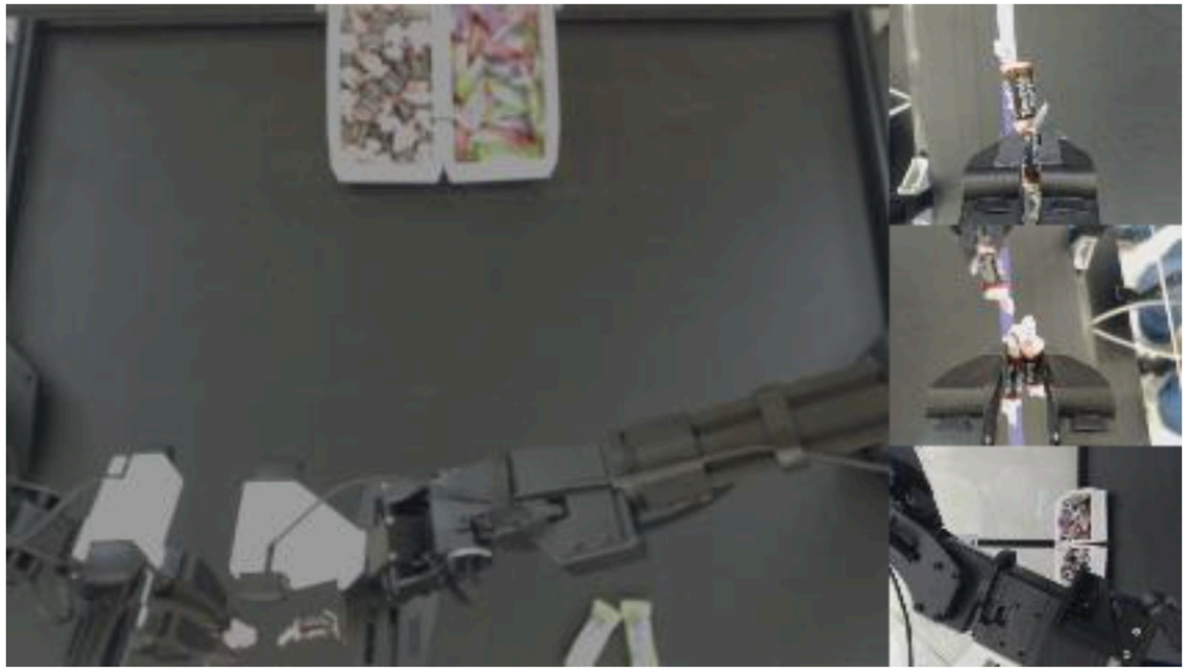

Supplement: Supplementary file 1 [file interface_v2.pdf]
